# Supplementary material for: Programmable System Call Security with eBPF
Source: arXiv:2302.10366 source file (2023-02-20)
Supplement: Supplementary file 1 [file appendix.tex]

\appendix
\section{Appendix}
\label{sec:appendix}

We discuss our helper function
    implementations that support checking argument values
    without being susceptible to TOCTTOU vulnerabilities~\cite{Canella_submission,Edge:deeparg:lwn}.
The key principle is to disallow userspace applications to
    modify the argument values as long as the values are used in a system call.

There are two basic approaches to implement such helpers without additional
    hardware support:
(1) making the data page write-protected or inaccessible from the user space by modifying protection bits in the page tables (e.g., RW bit and US bit), or
(2) copying the argument values to a protected memory region that can only be modified by the kernel.

For Seccomp-eBPF, we have implemented both approaches.
The first approach, called DPTI~\cite{Canella_submission},
    requires modifying protection bits in the page tables and flushing the corresponding TLB entry
    from all necessary CPU cores.
Moreover, it requires modifications to the
    page fault handler. The reason for that is that the data page can be accessed by
    concurrent threads for data on the page that is unrelated to the system call.
In the case of the modified RW bit, a write access by a concurrent thread causes a page fault while reads are permitted.
In the case of the modified US bit, both read and write accesses cause a page fault.
Hence, the page fault handler has to temporarily stall threads that perform a normally legitimate access to such modified pages.

For the second approach, we copy the argument values to dedicated kernel pages
    allocated for each thread, before entering Seccomp.
The kernel page is mapped to a userspace address, which is read-only
    to prevent TOCTTOU vulnerabilities.
We disable \texttt{VM\_MAYWRITE} of the page to prevent the user space from
  gaining the write permission (e.g., via \texttt{mprotect}).
% \claudio{this then requires disabling smap, right?
%  Why not make it a kernel address?
%  Because if it is a userspace address,
%  you have to take special care of mprotect as a concurrent threat can simply give write permissions to the page.
% I guess this would also break the semantic that a system call operates on userspace addresses, but this should be ok as long as data is then copied back to the userspace address before returning.}
Since the page is mapped in the user space, the kernel can maintain its
  original workflow of copying system call argument values from
  the user space.
So, we can directly use
    the existing user-memory reading helpers
    in the eBPF filter
    to access the argument values.
% The approach requires no TLB flush, improving performance.
Note that it needs to know how to copy the argument values for different
    system calls, i.e., it needs to know the argument semantics,
    such as the size of the object and the structures for nested pointers.
When a system call is invoked, an in-kernel hook is triggered to copy the
    argument values based on the semantic of the particular system call.
The hook is only enabled when an eBPF filter that uses the user-memory
    reading helpers are attached to the current thread.
% https://github.com/hckuo/kfuse-linux/tree/pb
% \tianyin{TODO: ask Austin to review this paragraph.}

% \austin{because the kernel would copy the memory from userspace and
% copy\_from\_user requires a user space memory (i am not sure if it is ok to remove
% the check)}

% Since the page is
% mapped to userspace, the hook modifies the argument to the new userspace address
% to not break \texttt{copy\_from\_user()} calls in the later code path and
% to support argument reading in userspace (e.g., seccomp user notifier, in this
% case, user notifier can not modify syscall arguments either).
% \tianyin{Is it correct that if I don't care about Seccomp Notifier, I don't need
%    it to be mapped to the user space? Or, putting another way, mapping
%    to userspace address is specific for Seccomp Notifier?}
% \austin{in theory yes, but it kinda breaks the assumption that system call
% arguments should be an userspace address? also the copy\_from\_user issue}

% Userspace applications have no access to the protected copy of arguments and
% only the protected copy will be used by both seccomp user notifier and the
% kernel. Therefore, TOCTTOU is mitigated.
